# Supplementary material for: Expressive Text-to-Image Generation with Rich Text
Source: arXiv:2304.06720 source file (2025-01-14)
Supplement: Supplementary file 1 [file supp.tex]

\documentclass[10pt,letterpaper]{article}

\input{setup/package}
\input{setup/macros}
\input{setup/symbols}
\input{setup/graphicspath}

\usepackage{iccv}

\iccvfinalcopy % *** Uncomment this line for the final submission

 % *** Enter the ICCV Paper ID here

% ==============================================================
% Main Document
% ==============================================================

\begin{document}
% \onecolumn
% {
% \Large
% \begin{center}
% \textbf{\noindent 3D Photography using Context-aware Layered Depth Inpainting\\Supplementary Material}
% \end{center}
% \maketitle
% }
% \title{Expressive Text-to-Image Generation with Rich Text \\Supplementary Material}
\title{Expressive Text-to-Image Generation with Rich Text Appendix}

% \twocolumn[{
% \renewcommand\twocolumn[1][]{#1}
% \maketitle
% }]
% \maketitle

% Main paper
\input{supp_content}

\clearpage
{\small
\bibliographystyle{ieee_fullname}
\bibliography{egbib}
}

\end{document}
